# Supplementary material for: QVIP: An ILP-based Formal Verification Approach for Quantized Neural Networks
Source: arXiv:2212.11138 source file (2022-12-10)
Supplement: Supplementary file 1 [file appendix-proofs.tex]

\section{Appendix}
